# Supplementary material for: A few algebraic problems in the theory of quantum entanglement
Source: arXiv:1305.2435 source file (2013-05-10)
Supplement: Supplementary file 1 [file appendixPPT3x3.tex]

\section{Sign constraints}\label{appconstraints} 
In this appendix, we give a list of constraints on the numbers listed in equations \eqref{numerkilista1} and \eqref{numerkilista2}. They are contained in Tables \ref{tabsigns3} and \ref{tabsigns2}. Some of the constraints are simple relations like $p-1>0\Rightarrow p>0$, but there are also more sophisticated ones. For example,
\begin{equation}\label{sophistic}
\left(r<0\land q-1<0\land r-ps>0\right)\Rightarrow qr-ps>0.
\end{equation}
Alternatively, the above formula can be written as
\begin{equation}\label{sophistic2}
\neg\left(r<0\land q-1<0\land r-ps>0\land qr-ps<0\right).
\end{equation}
This is also the convention we adopt in the following tables. For example, formula \eqref{sophistic2} corresponds to the following row in Table \ref{tabsigns3}.
\begin{equation}\nonumber
\scalebox{0.80}{
\begin{tabular}{|c|c|c|c|c|c|c|c|c|c|c|c|c|c|c|c|c|c|c|}
\hline
p&q&r&s&pp&qq&rr&ss&pq&rs&pr&ps&rq&qs&qrp&qrs&psq&rps&qrps\\
\hline
&&--&&&--&&&&&&&&&&&&+&--\\
\hline
\end{tabular}
}
\end{equation}
An explanation of the notation we used in the headers of the tables can be found in Appendix~\ref{appsignchoices}.
%As already explained in Appendix \ref{appsignchoices} the symbols $pp$, $qq$, $rr$ and $ss$ denote $p-1$, $q-1$, $r-1$ and $s-1$, respectively, while $pq$, $rs$, $pr$, $rq$, $qs$, $qrp$, $qrs$, $psq$, $rps$ and $qrps$ stand for $p-q$, $r-s$, $p-r$, $r-q$, $qr-p$, $qr-s$, $ps-q$, $r-ps$ and $qr-ps$, respectively.

\twocolumngrid

\begin{table}[b]\centering
%\begin{minipage}[b]{0.5\linewidth}
\scalebox{0.70}{
\begin{tabular}{|c|c|c|c|c|c|c|c|c|c|c|c|c|c|c|c|c|c|c|}
\hline
p&q&r&s&pp&qq&rr&ss&pq&rs&pr&ps&rq&qs&qrp&qrs&psq&rps&qrps\\
\hline
&&+&&&+&&&&+&&&&&&--&&&\\
&+&&&&&+&&&&&&&+&&--&&&\\
&&+&&&--&&&&--&&&&&&+&&&\\
&+&&&&&--&&&&&&&--&&+&&&\\
&&&+&+&&&&&&&&&--&&&--&&\\
+&&&&&&&+&+&&&&&&&&--&&\\
&&&+&--&&&&&&&&&+&&&+&&\\
+&&&&&&&--&--&&&&&&&&+&&\\
&+&&&&&+&&--&&&&&&--&&&&\\
&&+&&&+&&&&&--&&&&--&&&&\\
&+&&&&&--&&+&&&&&&+&&&&\\
&&+&&&--&&&&&+&&&&+&&&&\\
+&&&&&&&+&&&+&&&&&&&+&\\
&&&+&+&&&&&--&&&&&&&&+&\\
+&&&&&&&--&&&--&&&&&&&--&\\
&&&+&--&&&&&+&&&&&&&&--&\\
&&&+&--&&&&&&&&&&&+&&&--\\
&&&+&+&&&&&&&&&&&--&&&+\\
&+&&&&&+&&&&&&&&&&--&&--\\
&+&&&&&--&&&&&&&&&&+&&+\\
+&&&&&&&--&&&&&&&+&&&&--\\
+&&&&&&&+&&&&&&&--&&&&+\\
&&+&&&+&&&&&&&&&&&&+&--\\
&&+&&&--&&&&&&&&&&&&--&+\\
&&--&&&+&&&&--&&&&&&+&&&\\
&&--&&&--&&&&+&&&&&&--&&&\\
&--&&&&&--&&&&&&&+&&--&&&\\
&--&&&&&+&&&&&&&--&&+&&&\\
&&&--&--&&&&&&&&&--&&&--&&\\
--&&&&&&&--&+&&&&&&&&--&&\\
&&&--&+&&&&&&&&&+&&&+&&\\
--&&&&&&&+&--&&&&&&&&+&&\\
&--&&&&&--&&--&&&&&&--&&&&\\
&&--&&&--&&&&&--&&&&--&&&&\\
&--&&&&&+&&+&&&&&&+&&&&\\
&&--&&&+&&&&&+&&&&+&&&&\\
--&&&&&&&+&&&--&&&&&&&--&\\
&&&--&+&&&&&+&&&&&&&&--&\\
--&&&&&&&--&&&+&&&&&&&+&\\
&&&--&--&&&&&--&&&&&&&&+&\\
\hline
\end{tabular}
}
\vskip 2 pt
\caption{Non-admissible sign choices. Part I.}
\label{tabsigns3}
\end{table}
%\end{minipage}\hskip 0.5 cm
%\begin{minipage}[b]{0.5\linewidth}%\centering
\begin{table}[b]\centering
\scalebox{0.7}{
\begin{tabular}{|c|c|c|c|c|c|c|c|c|c|c|c|c|c|c|c|c|c|c|}
\hline
p&q&r&s&pp&qq&rr&ss&pq&rs&pr&ps&rq&qs&qrp&qrs&psq&rps&qrps\\
%p&q&r&s&pp&qq&rr&ss&pq&rs\\
\hline
&&&--&+&&&&&&&&&&&+&&&--\\
&&&--&--&&&&&&&&&&&--&&&+\\
&--&&&&&--&&&&&&&&&&--&&--\\
&--&&&&&+&&&&&&&&&&+&&+\\
--&&&&&&&+&&&&&&&+&&&&--\\
--&&&&&&&--&&&&&&&--&&&&+\\
&&--&&&--&&&&&&&&&&&&+&--\\
&&--&&&+&&&&&&&&&&&&--&+\\
%tu przełożone
--&&&&+&&&&&&&&&&&&&&\\
&--&&&&+&&&&&&&&&&&&&\\
&&--&&&&+&&&&&&&&&&&&\\
&&&--&&&&+&&&&&&&&&&&\\
--&+&&&&&&&+&&&&&&&&&&\\
+&--&&&&&&&--&&&&&&&&&&\\
&&+&--&&&&&&--&&&&&&&&&\\
&&--&+&&&&&&+&&&&&&&&&\\
&&&&--&+&&&+&&&&&&&&&&\\
&&&&+&--&&&--&&&&&&&&&&\\
&&&&&&--&+&&+&&&&&&&&&\\
&&&&&&+&--&&--&&&&&&&&&\\
%\hline
%\end{tabular}
%}
%\vskip 2 pt
%\caption{Non-admissible sign choices. Part I.}
%\label{tabsigns1}
%\end{table}
%
%\begin{table}[ht]
%\scalebox{0.9}{
%\begin{tabular}{|c|c|c|c|c|c|c|c|c|c|c|c|c|c|c|c|c|c|c|}
%\hline
%p&q&r&s&pp&qq&rr&ss&pq&rs&pr&ps&rq&qs&qrp&qrs&psq&rps&qrps\\
%\hline
&&&&&--&&+&&&&&&+&&&&&\\
&--&&+&&&&&&&&&&+&&&&&\\
&+&&--&&&&&&&&&&--&&&&&\\
&&&&&+&&--&&&&&&--&&&&&\\
--&&+&&&&&&&&+&&&&&&&&\\
&&&&--&&+&&&&+&&&&&&&&\\
+&&--&&&&&&&&--&&&&&&&&\\
&&&&+&&--&&&&--&&&&&&&&\\
&+&--&&&&&&&&&&+&&&&&&\\
&&&&&+&--&&&&&&+&&&&&&\\
&--&+&&&&&&&&&&--&&&&&&\\
&&&&&--&+&&&&&&--&&&&&&\\
--&&&+&&&&&&&&+&&&&&&&\\
&&&&--&&&+&&&&+&&&&&&&\\
+&&&--&&&&&&&&--&&&&&&&\\
&&&&+&&&--&&&&--&&&&&&&\\
\hline
\end{tabular}
}
%\end{minipage}
\vskip 2 pt
\caption{Non-admissible sign choices. Part~II.}
\label{tabsigns2}
\end{table}
